# Supplementary material for: Distilling Optimal Neural Networks: Rapid Search in Diverse Spaces
Source: arXiv:2012.08859 source file (2021-08-27)
Supplement: Supplementary file 1 [file 01_ablation.tex]

\section{Ablation Study} \label{sec:ablation}
\subsection{Block Transplantation and Blockwise Knowledge Distillation}
Discuss impact of learning schedule (learning rate, optimizer, number of steps, loss function).

\subsection{Training schemes for Blockwise Knowledge Distillation}
Discuss impact of learning schedule (learning rate, optimizer, number of steps, loss function).

\subsection{Choice of Mother Network}

\begin{figure*}[!h]
\centering
\begin{subfigure}{.45\textwidth}
  \centering
  \includegraphics[width=.90\linewidth]{./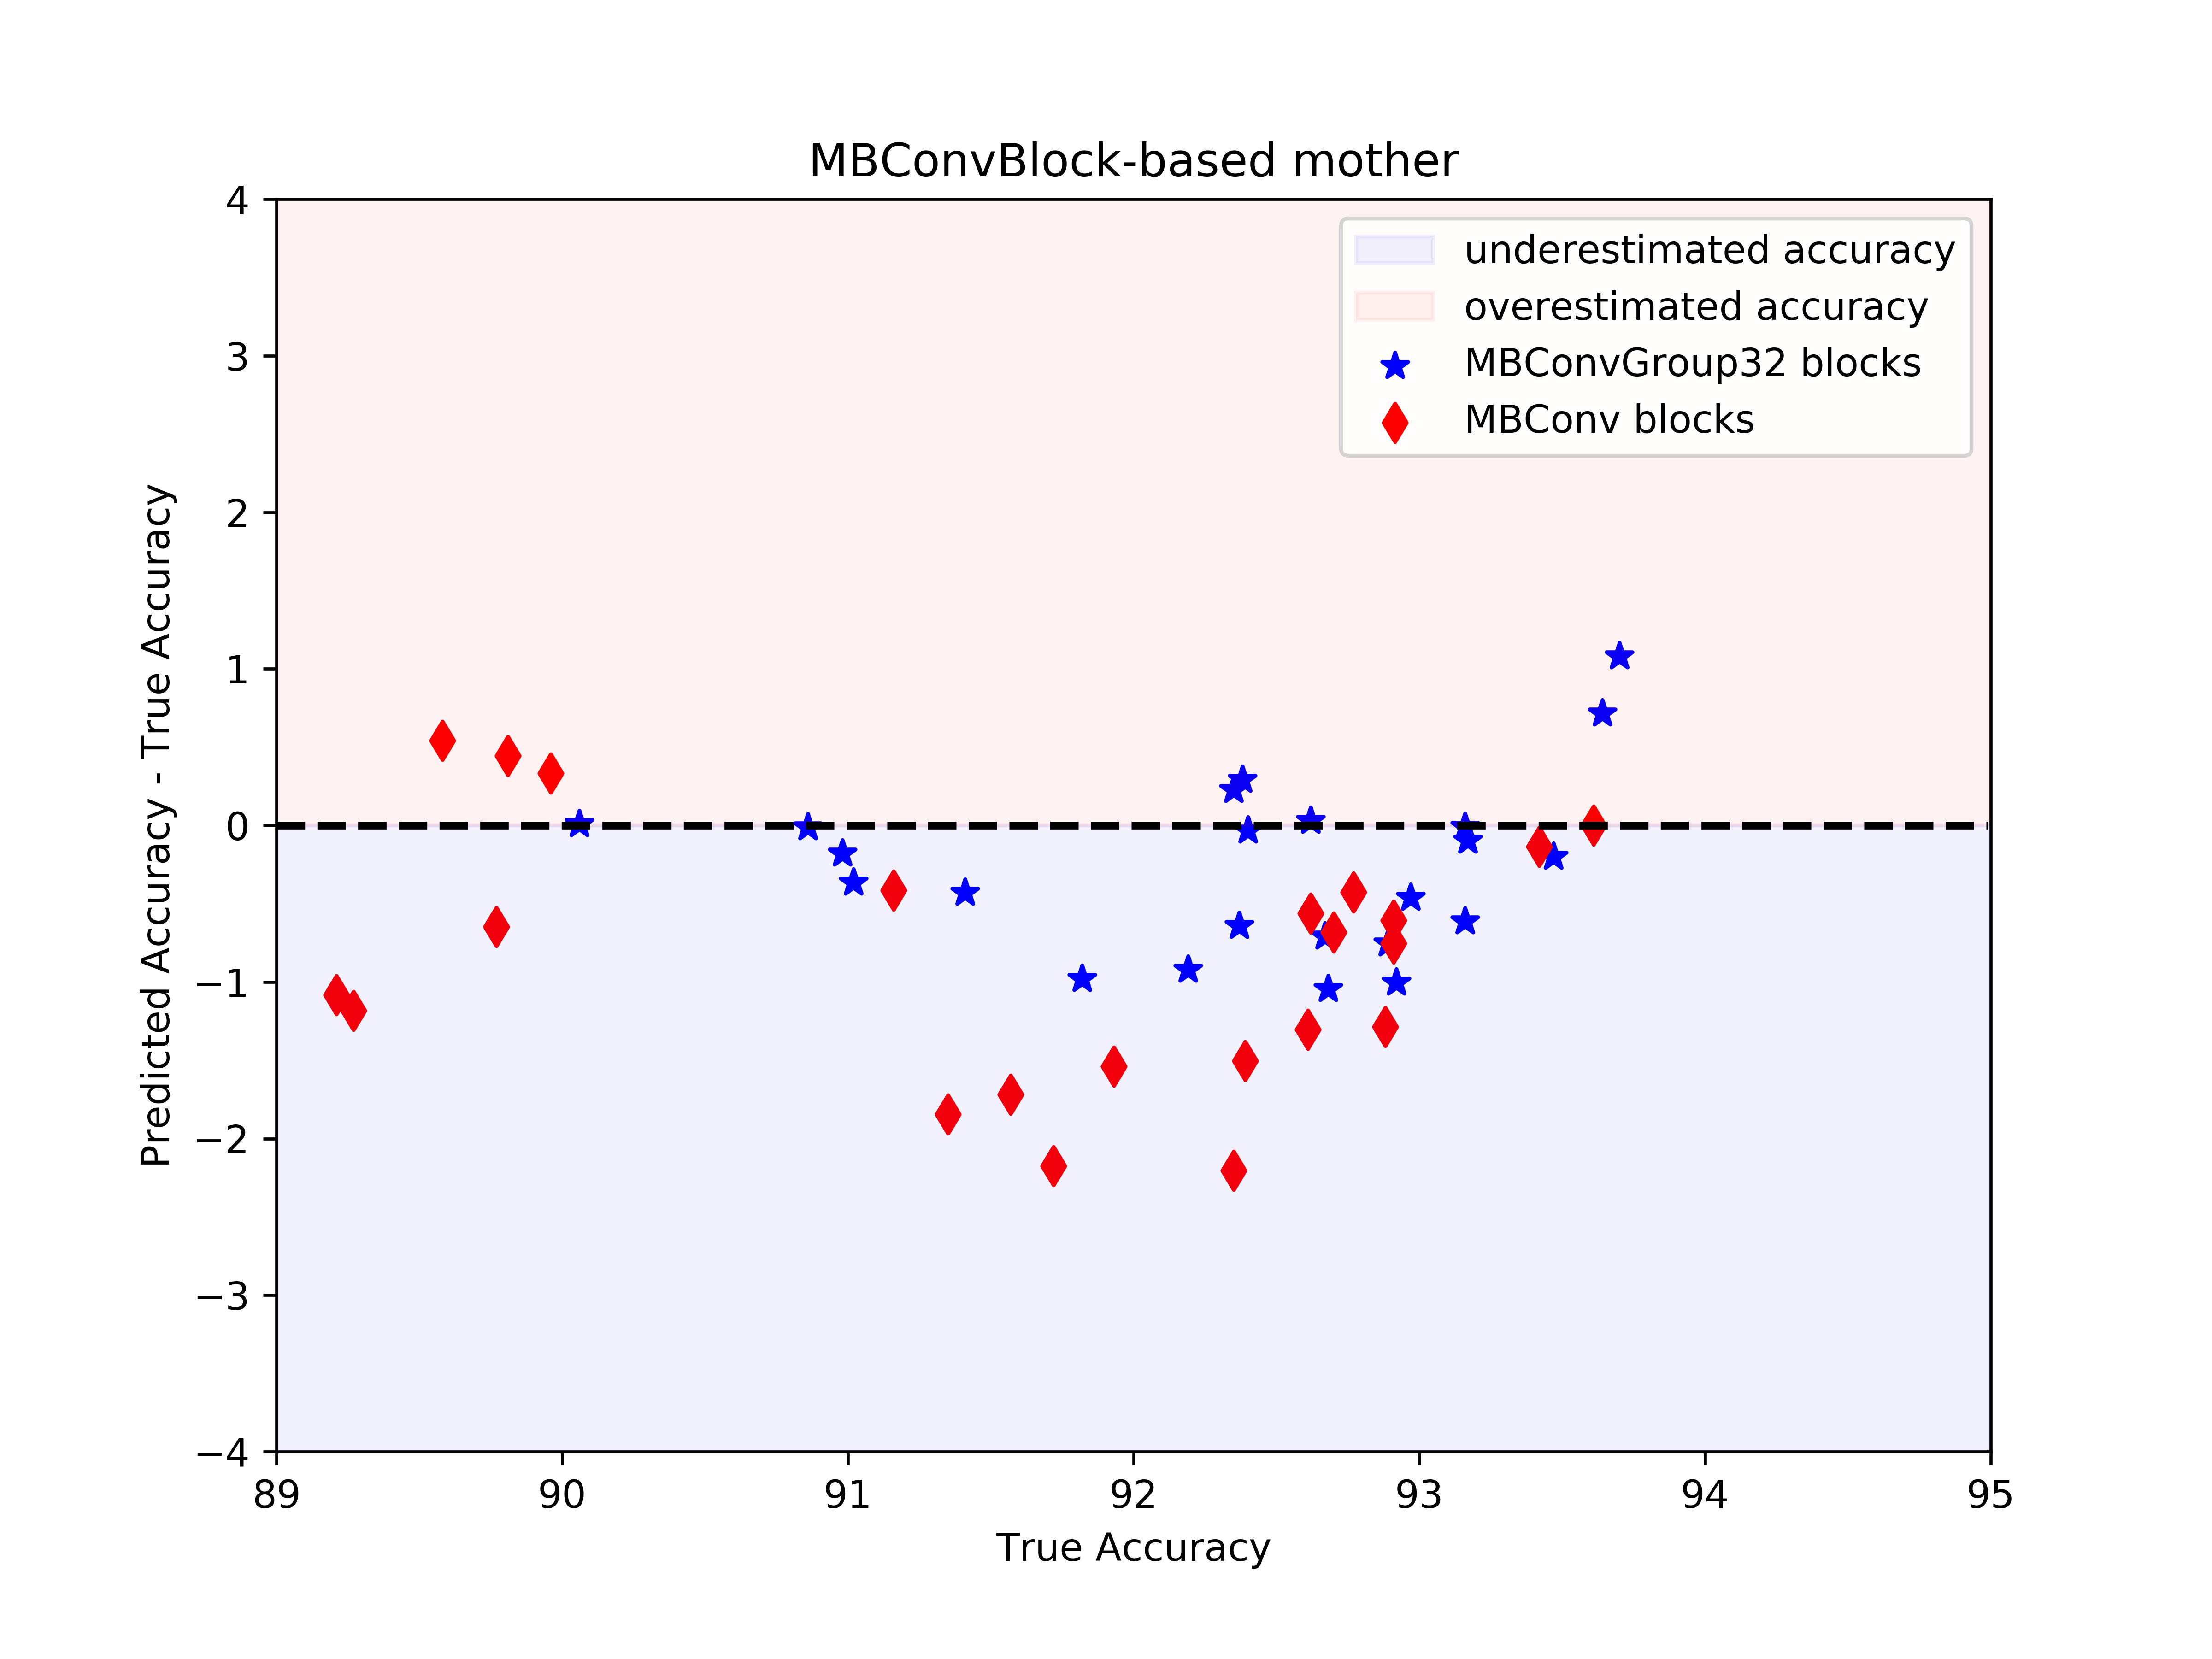}
  \label{fig:params}
\end{subfigure}
\begin{subfigure}{.45\textwidth}
  \centering
  \includegraphics[width=.90\linewidth]{./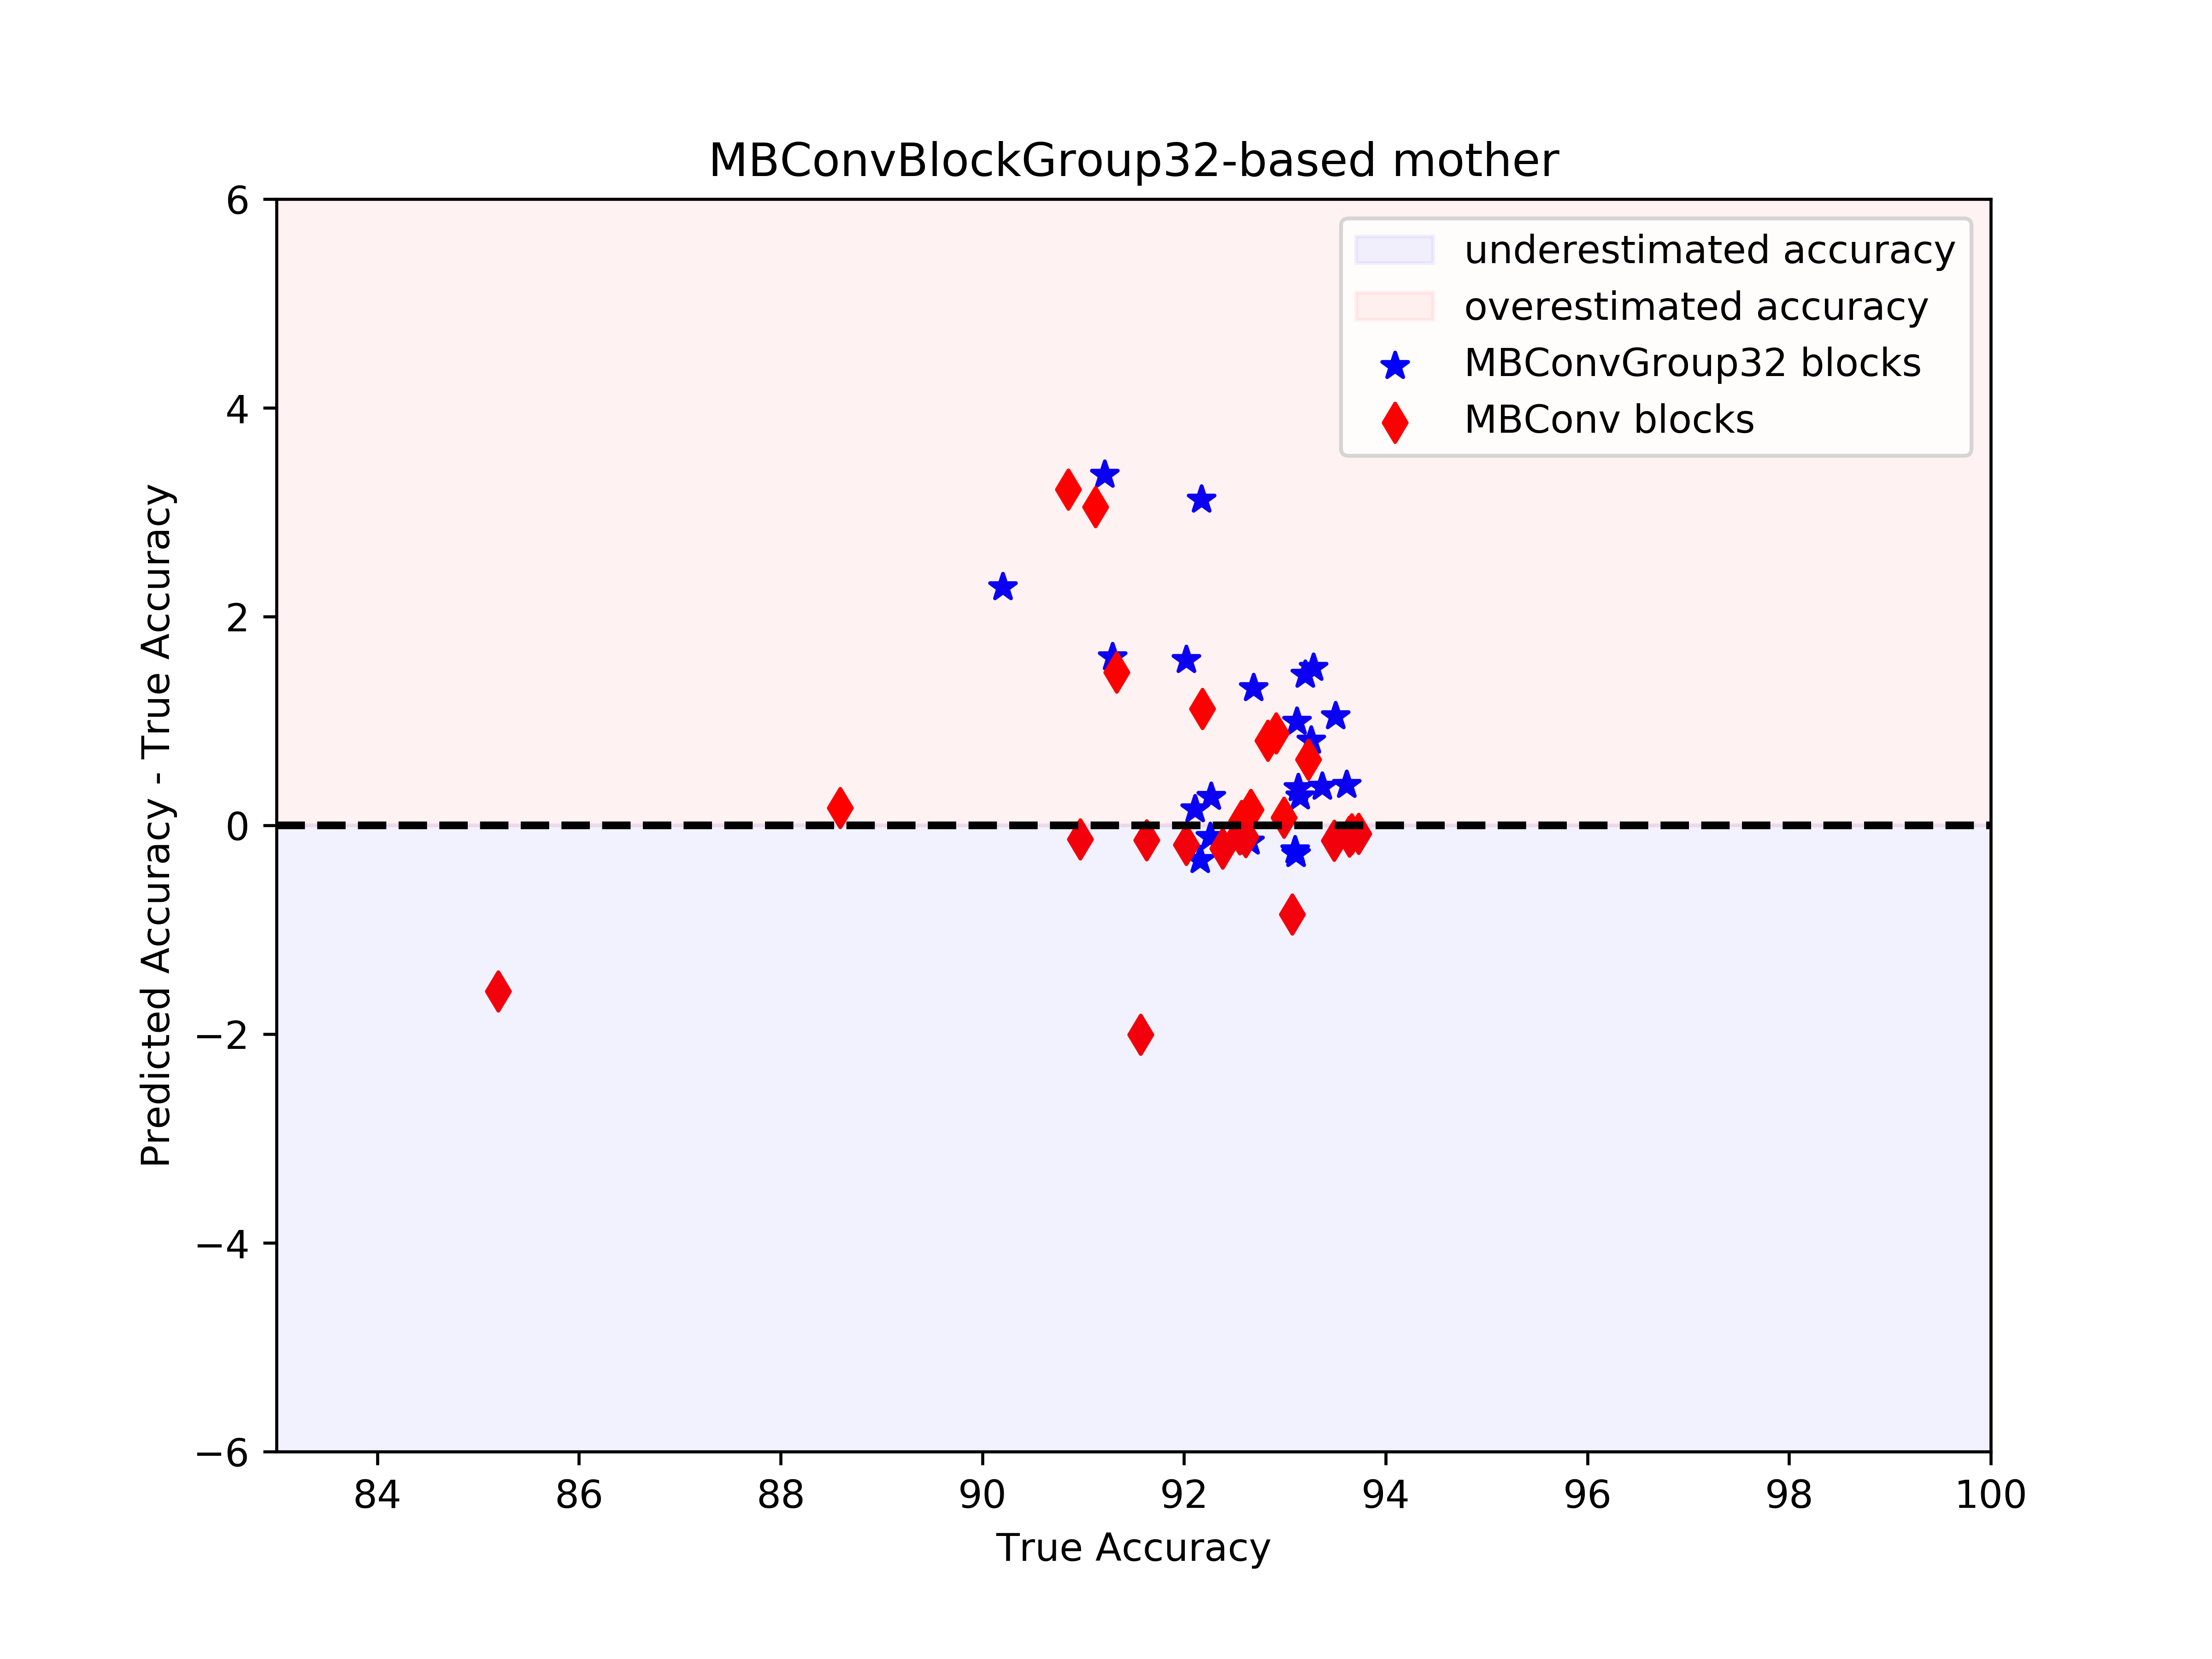}
  \label{fig:flops}
\end{subfigure}
\caption{Performance of accuracy predictors on different search spaces for MBConvBlock (left) and MBConvBlockGroup32 (right) mother networks.}
\label{fig:cifar10}
\end{figure*}

One of the most important choices to make before doing the whole QUARTS procedure is choosing a mother network. Since it will be used at every step of the procedure, choosing a wrong one might result in multiple issues: (1) blocks trained with knowledge distillation might not reach satisfying accuracy; (2) built accuracy predictor might give a wrong estimate for the selected search space; (3) due to knowledge distillation procedure in the finetuning, resulting models can have lower accuracy compared to using a better teacher.

The main assumption being used throughout the paper is that the best teacher is the largest one. This is in line with previous works \cite{yang2018knowledge,lan2018knowledge,yim2017agift}. However, another line of research \cite{cho2019efficacy} has shown that the biggest teachers might hinder the performance of students if those can't reach the same capacity as the teacher. We have not observed that in any of our experiments and we hypothesize that it is due to the blockwise training procedure which leads to easier optimization. Since we are trying to approximate per-block function it ends up being easier than approximating full model. 

To confirm our hypothesis even further, we conduct a set of experiments where we use two different mother networks as teachers - a larger one (MBConvBlockGroup32-based) and a smaller one (MBConvBlock-based). We then use those to build two accuracy models - one per teacher and assess accuracies of models consisting fully of  blocks and MBConvGroup32 blocks. As you can see in \ref{fig:cifar10}, using larger model allows for a good estimate for both MBConv and MBConvGroup32 models. However, when using smaller model, MBConvGroup32 models end up being highly underestimated since smaller teacher prevents models from learning further during blockwise kd training.

This confirms that when training on a new search space, the largest model in this search space should be used as a teacher.
