# Supplementary material for: Distilling Optimal Neural Networks: Rapid Search in Diverse Spaces
Source: arXiv:2012.08859 source file (2021-08-27)
Supplement: Supplementary file 2 [file supplementary_finetuning_speed.tex]

\begin{figure}[t]
\centering
 \includegraphics[width=.99\linewidth]{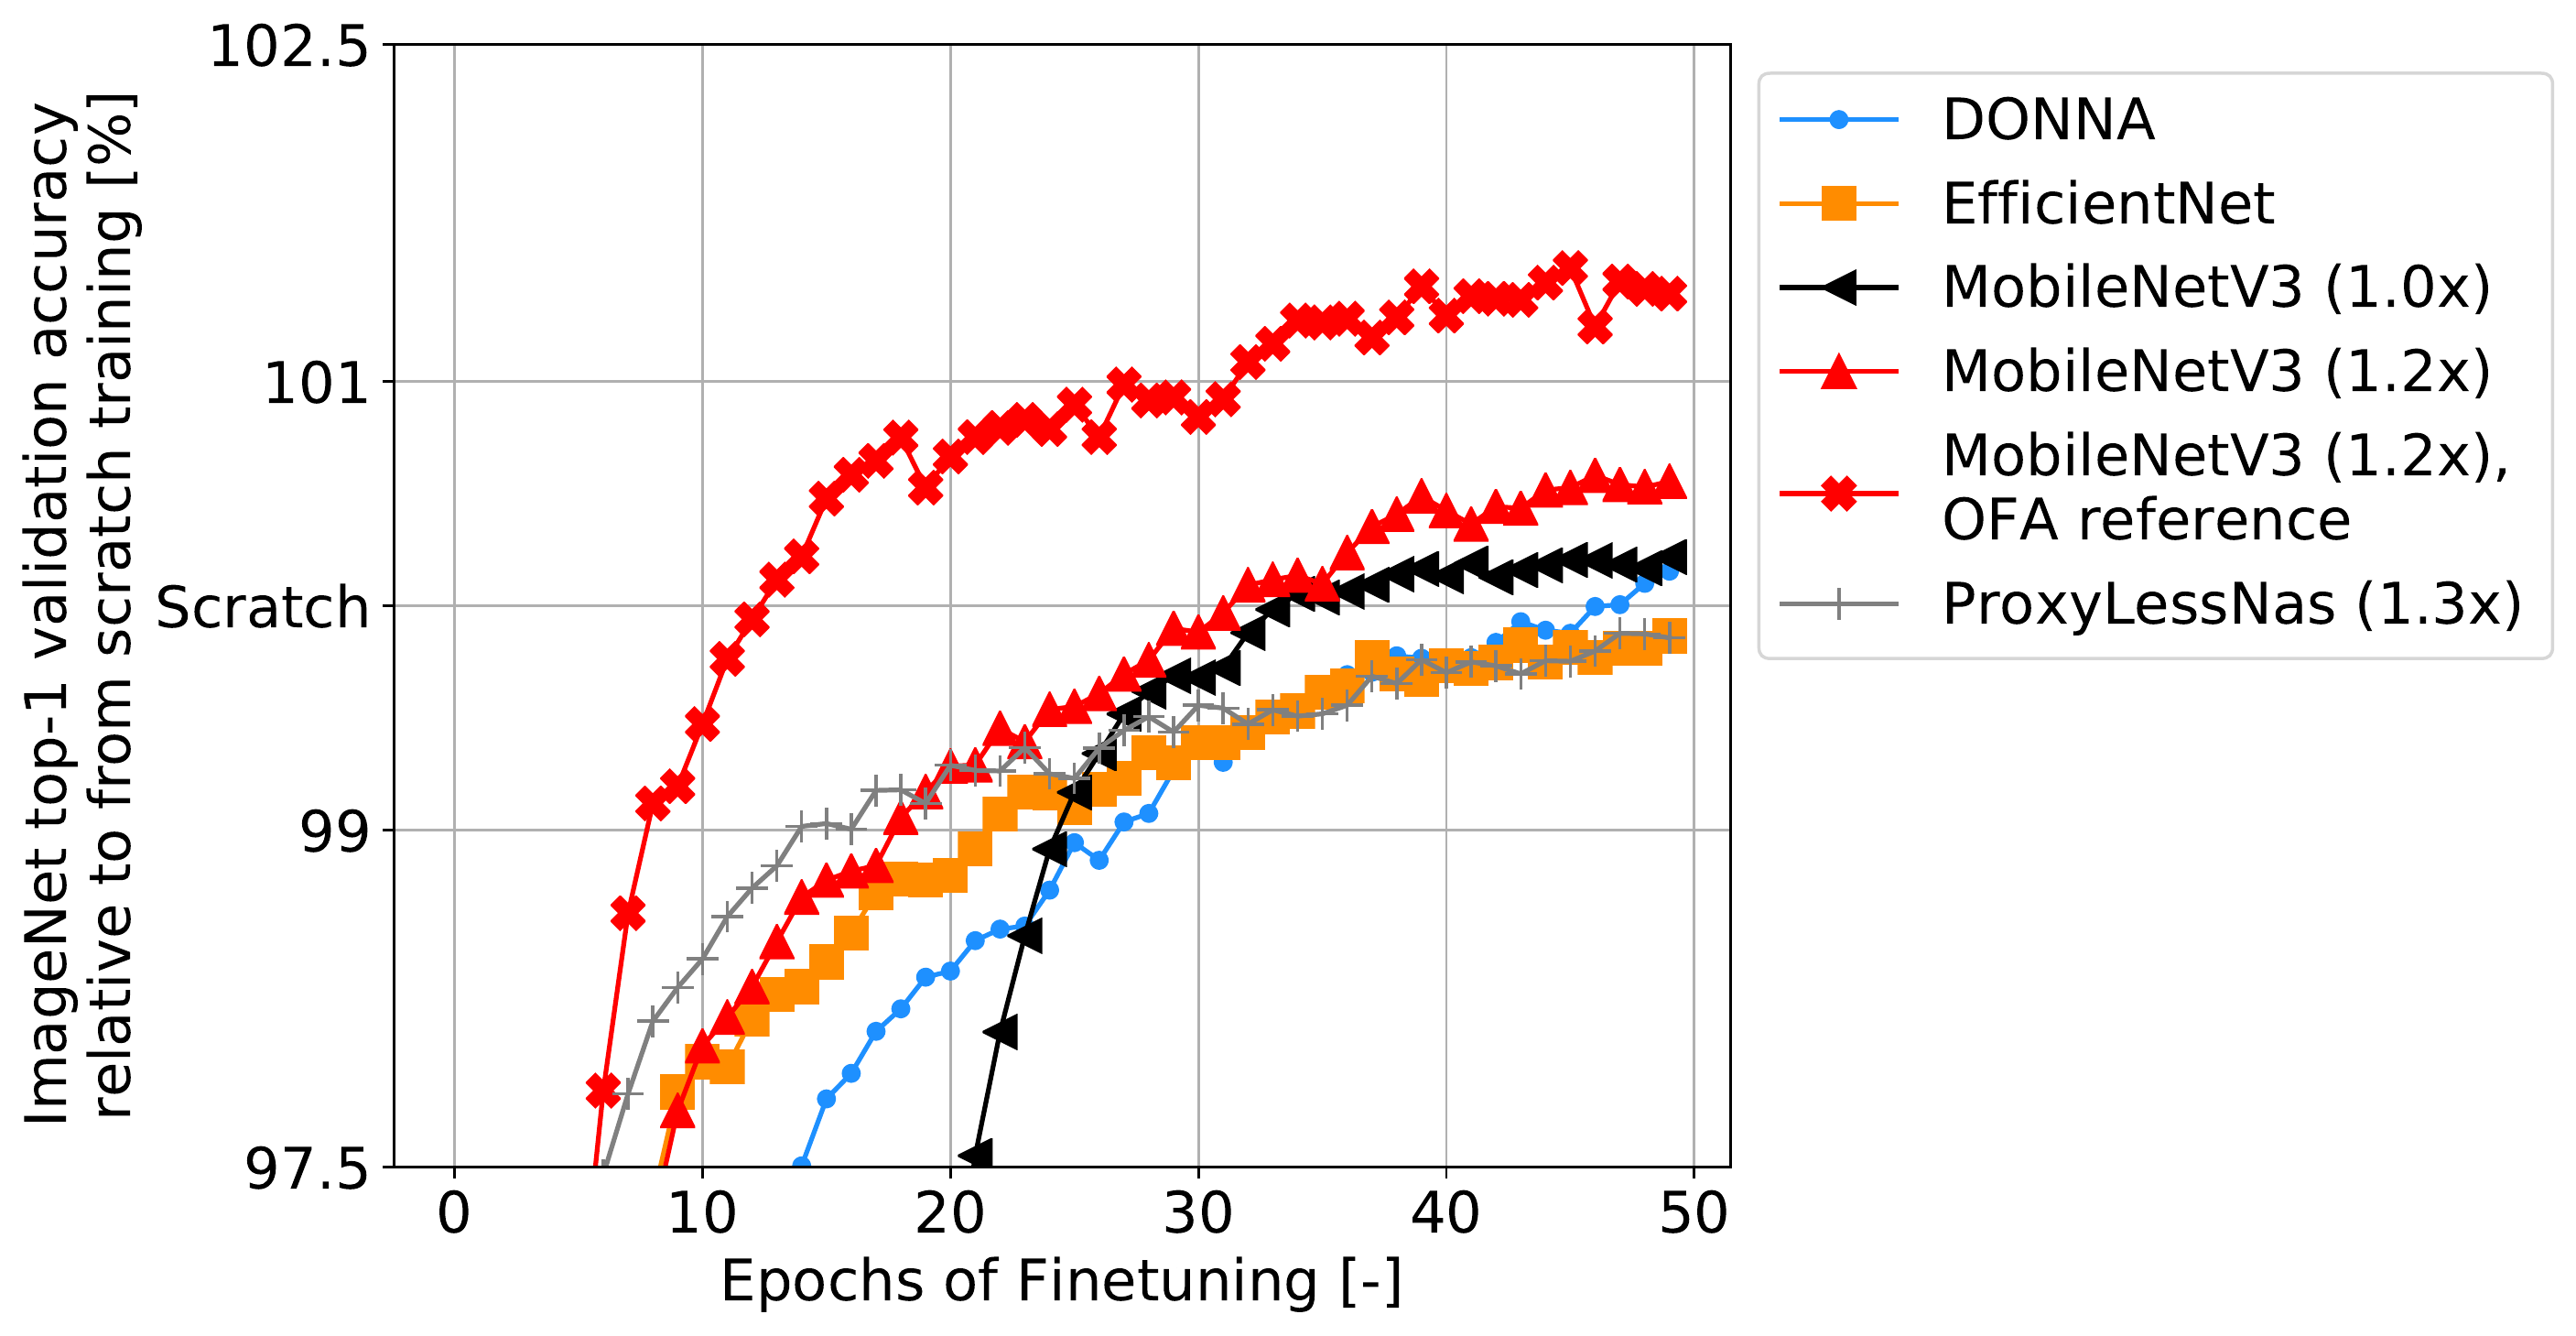}
\caption{Speed at which BKD-initialized subsampled models can be finetuned for different search spaces. Models in ~\methodname, EfficientNet and ProxyLessNas (1.3$\times$) converge to the accuracy of 450-epoch from scratch training in less than 50 epochs using the BKD initialization point, a $9\times speedup$. Models in the MobileNetV3 search space converge in about 30 epochs, a $15\times$ speedup. If the supernet from OFA~\cite{ofa_repo,ofa} is used as a reference model and teacher model in the \methodname pipeline for MobileNetV3 (1.2$\times$), from-scratch 450 epoch accuracy is even achieved in less than 15 epochs, a $30\times$ speed up.}
\label{fig:supplementary/finetuning-speed}
\end{figure}
