# Supplementary material for: Distilling Optimal Neural Networks: Rapid Search in Diverse Spaces
Source: arXiv:2012.08859 source file (2021-08-27)
Supplement: Supplementary file 3 [file supplementary_flops_params_gpu.tex]

\begin{figure*}[t]
\centering
 \includegraphics[width=.99\linewidth]{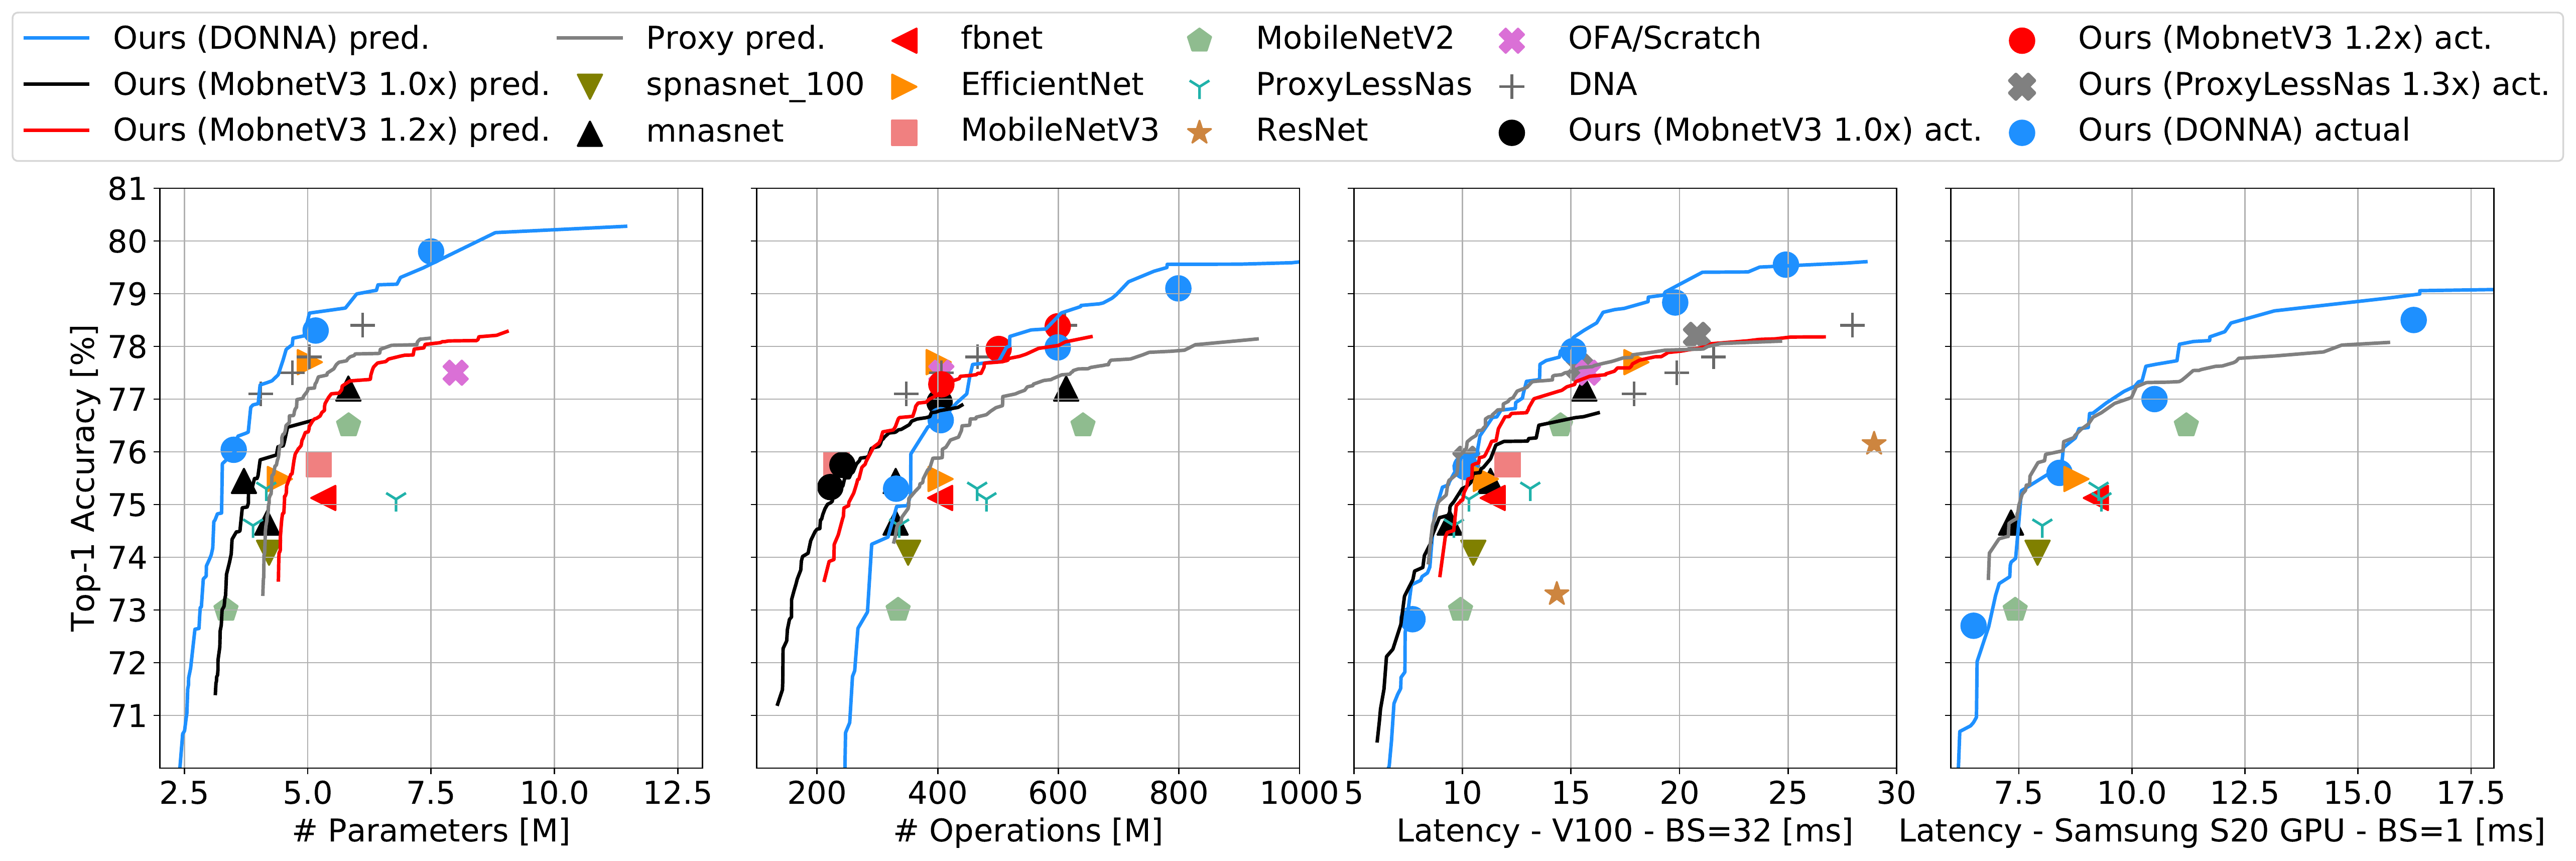}
\caption{Trendlines and models found by \methodname~optimizing for the number of parameters (left), the number of operations (mid left), inference time on an Nvidia V100 GPU (mid right) and a commercially available Samsung S20 smartphone GPU (right). Best viewed in color.}
\label{fig:supplementary/search-space-overview}
\end{figure*}
